# Supplementary material for: Joint Wireless and Edge Computing Resource Management with Dynamic Network Slice Selection
Source: arXiv:2001.07964 source file (2020-01-22)
Supplement: Supplementary file 1 [file appendix.tex]

\begin{lemma}\label{lemm::closed_form_exp_slices}
	Let us consider the following problem 
\begin{eqnarray}
 &\rev{\min \nolimits_{\bf{x}} \sum \nolimits_{f \in \mathcal{F}} \sum \nolimits_{s \in \mathcal{S}} \frac{1}{b_{f}^s} \big(\sum \nolimits_{i \in \mathcal{K}_{f,s}}\frac{A_{i,f}^s}{x_{i,f}^s}\big)}\label{eq::slices_objective}\\
 \textrm{s.t.}& x_{i,f}^s \geq 0, \forall i \in \mathcal{K}_{f,s}, \forall f \in \mathcal{F},  \forall s \in \mathcal{S}, \label{eq::constraint_positive_variable_constraint_slices}\\
  &\rev{\sum \nolimits_{j \in \mathcal{K}_{f,s}}  x_{j,f}^s \leq 1, \forall f \in \mathcal{F},\forall s \in \mathcal{S},} \hspace{0.4cm} \label{eq::constraint_sum_of_variables_slices}
 \end{eqnarray}
 where $A_{i,f}^s \!\in\! \mathbb{R}_{\geq 0}$, $b_{f}^s \!\in\! \mathbb{R}_{> 0}$ and $\mathcal{F}$, $\mathcal{S}$ and $\mathcal{K} = \cup_{f \in \mathcal{F}, s \in \mathcal{S}}\mathcal{K}_{f,s}$ are non-empty sets.
 Then, closed form solution for (\ref{eq::slices_objective})-(\ref{eq::constraint_sum_of_variables_slices}) is given by 
 \begin{equation}\label{eq::optimal_coef_slices}
     x_{i,f}^{s*} = \frac{\sqrt{A_{i,f}^s}}{\sum \nolimits_{j \in \mathcal{K}_{f,s}}\sqrt{A_{j,f}^s}}, \forall i \in \mathcal{K}_{f,s}, \forall f \in \mathcal{F}, \forall s \in \mathcal{S}.
 \end{equation}
 \end{lemma}
\begin{proof}
By inspecting the leading minors of the Hessian matrix of the objective function it is easy to show that the matrix is positive semidefinite on the domain defined by (\ref{eq::constraint_positive_variable_constraint_slices})-(\ref{eq::constraint_sum_of_variables_slices}), and thus problem (\ref{eq::slices_objective})-(\ref{eq::constraint_sum_of_variables_slices}) is convex. Therefore, the optimal solution of the problem must satisfy the Karush–Kuhn–Tucker (KKT)
conditions and thus we can formulate the corresponding Lagrangian dual problem. \rev{To do so, let us introduce non-negative Lagrange multiplier vectors $\vardualeqconstraintcomvec = (\vardualeqconstraintcom_{i,f}^s)_{i \in \mathcal{K}_{f,s},f \in \mathcal{F}, s \in \mathcal{S}}$ and $\vardualneqconstraintcom = (\vardualneqconstraintcom_{f}^s)_{f \in \mathcal{F}, s \in \mathcal{S}}$ for constraints (\ref{eq::constraint_positive_variable_constraint_slices}) and (\ref{eq::constraint_sum_of_variables_slices}), respectively.} Next, let us define the Lagrangian dual problem corresponding to problem (\ref{eq::slices_objective})-(\ref{eq::constraint_sum_of_variables_slices}) as \rev{$\max \limits_{\vardualeqconstraintcomvec \succeq 0, \vardualneqconstraintcomvec\succeq 0} \min \limits_{\bf{x} \succeq 0} \varlagrangian(\bf{x},\vardualneqconstraintcomvec,\vardualeqconstraintcomvec)$, where the Lagrangian is given by}
\vspace{-0.3cm}
\begin{eqnarray}\label{eq::lagrangian_function_general}\nonumber
 &\varlagrangian(\bf{x},\vardualneqconstraintcomvec,\vardualeqconstraintcomvec)= \rev{ \sum \limits_{f \in \mathcal{F}} \sum \limits_{s \in \mathcal{S}} \frac{1}{b_{f}^s} \big(\sum \limits_{i \in \mathcal{K}_{f,s}}\frac{A_{i,f}^s}{x_{i,f}^s}\big)}+\\\nonumber
  &\hspace{-0.2cm}\sum \limits_{f \in \mathcal{F}} \sum \limits_{s \in \mathcal{S}}\! \vardualneqconstraintcom_{f}^s \big(\sum \limits_{j \in \mathcal{K}_{f,s}}x_{j,f}^s - 1) \big)  - \sum \limits_{f \in \mathcal{F}}\sum \limits_{s \in \mathcal{S}} \sum \limits_{j \in \mathcal{K}_{f,s}} \vardualeqconstraintcom_{j,f}^s x_{j,f}^s.\nonumber
 \end{eqnarray}
 By finding the first order derivatives of $\varlagrangian(\bf{x},\vardualneqconstraintcomvec,\vardualeqconstraintcomvec)$ with respect to the primal variables $x_{i,f}^s$, we can express the KKT stationarity conditions as \rev{$\frac{A_{i,f}^s}{b_{f}^s (x_{i,f}^s)^2} \!\!=\!\! \vardualneqconstraintcom_{f}^s \!-\! \vardualeqconstraintcom_{i,f}^s, \forall f \!\in\! \mathcal{F}, \forall s \!\in\! \mathcal{S}, \forall i \!\in\! \mathcal{K}_{f,s}$.}
\rev{From the KKT dual feasibility conditions $\vardualeqconstraintcomvec \!\succeq\! 0$ and complementary slackness conditions $-\vardualeqconstraintcom_{i,f}^sx_{i,f}^s \!=\! 0$ we obtain that $\vardualeqconstraintcom_{i,f}^s \!=\! 0$ must hold for every $f \!\in\! \mathcal{F}$, $s \!\in\! \mathcal{S}$, $i \!\in\! \mathcal{K}_{f,s}$ as otherwise $x_{i,f}^s \!=\! 0$ would lead to infinite value of the objective function. Therefore, from the the KKT stationarity conditions, we obtain $x_{i,f}^s = \sqrt{\frac{A_{i,f}^s}{b_{f}^s\vardualneqconstraintcom_{f}^s}}$. By substituting $x_{j,f}^s = \sqrt{\frac{A_{j,f}^s}{b_{f}^s\vardualneqconstraintcom_{f}^s}}$ into complementary slackness conditions $\vardualneqconstraintcom_{f}^s(\sum_{j \in \mathcal{K}_{f,s}}x_{j,f}^s - 1) = 0$, we obtain that $\vardualneqconstraintcom_{f}^s=\frac{1}{b_{f}^s}\big(\sum_{j \in \mathcal{K}_{f,s}}\sqrt{A_{j,f}^s}\big)^2$.  Finally, from $x_{i,f}^s = \sqrt{\frac{A_{i,f}^s}{b_{f}^s \vardualneqconstraintcom_{f}^s}}$ we obtain the expression~(\ref{eq::optimal_coef_slices}) for coefficients $x_{i,f}^{s*}$, which proves the result.}
\end{proof}

\rev{
\begin{lemma}\label{lemm::closed_form_exp_SRO}
	Let us consider the following problem 
\begin{eqnarray}
&\rev{\min \nolimits_{\bf{b}} \sum \nolimits_{f \in \mathcal{F}} \sum \nolimits_{s \in \mathcal{S}} \frac{1}{b_{f}^s} \big(\sum \nolimits_{i \in \mathcal{K}_{f,s}}\sqrt{A_{i,f}^s}\big)^2}\label{eq::SRO_objective}\\
\textrm{s.t.}& b_{f}^s \geq 0, \forall f \in \mathcal{F},  \forall s \in \mathcal{S}, \label{eq::constraint_positive_variable_constraint_SRO}\\
&\rev{\sum \nolimits_{s^\prime \in \mathcal{S}}  b_{f}^{s^{\prime}} \leq 1, \forall f \in \mathcal{F},} \hspace{0.4cm} \label{eq::constraint_sum_of_variables_SRO}
\end{eqnarray}
	obtained by substituting (\ref{eq::optimal_coef_slices}) into (\ref{eq::slices_objective}) and minimizing the obtained objective function w.r.t. $\bf{b}$.
	Then, closed form solution for (\ref{eq::SRO_objective})-(\ref{eq::constraint_sum_of_variables_SRO}) is given by 
	\begin{equation}\label{eq::optimal_coef_SRO}
	b_f^{s*} = \frac{\sum \nolimits_{i \in \mathcal{K}_{f,s}}\sqrt{A_{i,f}^s}}{\sum \nolimits_{s^\prime \in \mathcal{S}}\sum \nolimits_{i \in \mathcal{K}_{f,s^\prime}}\sqrt{A_{i,f}^{s^\prime}}}, \forall f \in \mathcal{F}, \forall s \in \mathcal{S}.
	\end{equation}
\end{lemma}
\begin{proof}
	Observe that the problem (\ref{eq::SRO_objective})-(\ref{eq::constraint_sum_of_variables_SRO}) has the same form as the problem (\ref{eq::SRO_objective})-(\ref{eq::constraint_sum_of_variables_SRO}). Therefore, by following the proof of Lemma~\ref{lemm::closed_form_exp_slices} we can obtain the
	expression (\ref{eq::optimal_coef_SRO}) for coefficients $	b_f^{s*}$, which proves
	the result.
\end{proof}
\begin{lemma}\label{lemm::closed_form_exp_general}
	Let us consider the following problem 
\begin{eqnarray}
 &\rev{\min \nolimits_{\bf{x}, \bf{b}} \sum \nolimits_{f \in \mathcal{F}} \sum \nolimits_{s \in \mathcal{S}} \frac{1}{b_{f}^s} \big(\sum \nolimits_{i \in \mathcal{K}_{f,s}}\frac{A_{i,f}^s}{x_{i,f}^s}\big)}\label{eq::general_objective}\\
 \textrm{s.t.}& (\ref{eq::constraint_positive_variable_constraint_slices}), (\ref{eq::constraint_sum_of_variables_slices}), (\ref{eq::constraint_positive_variable_constraint_SRO}), (\ref{eq::constraint_sum_of_variables_SRO}).   \label{eq::constraints_genral}
 \end{eqnarray}
	Then, closed form solution for (\ref{eq::general_objective})-(\ref{eq::constraints_genral}) is given by (\ref{eq::optimal_coef_slices}) and (\ref{eq::optimal_coef_SRO}).
\end{lemma}
\begin{proof}
First, let us define the Lagrangian for the problem (\label{ref::closed_form_exp_general})-(\ref{eq::constraints_genral}) as 
$$\varlagrangian(\bf{x}, \bf{b}, \vardualneqconstraintcomvec,\vardualeqconstraintcomvec) = \varlagrangian(\bf{x},\vardualneqconstraintcomvec,\vardualeqconstraintcomvec) + \sum_{f \in \mathcal{F}} \beta_f (\sum_{s^\prime \in \mathcal{S}}  b_{f}^{s^{\prime}} - 1) - \sum_{f \in \mathcal{F}} \sum_{s^\prime \in \mathcal{S}} \delta_f^{s^\prime}b_{f}^{s^{\prime}}$$
observe that we can obtain the expression~(\ref{eq::optimal_coef_slices}) for coefficients $x_{i,f}^{s*}$ by following the proof of Lemma~\ref{lemm::closed_form_exp_slices}. Next, by finding the first order derivatives of $\varlagrangian(\bf{x}, \bf{b}, \vardualneqconstraintcomvec,\vardualeqconstraintcomvec) = \varlagrangian(\bf{x},\vardualneqconstraintcomvec,\vardualeqconstraintcomvec) + \sum_{f \in \mathcal{F}} \beta_f (\sum_{s^\prime \in \mathcal{S}}  b_{f}^{s^{\prime}} - 1) - \sum_{f \in \mathcal{F}} \sum_{s^\prime \in \mathcal{S}} \delta_f^{s^\prime}b_{f}^{s^{\prime}}$ with respect to the primal variables $x_{i,f}^s$, we can express the KKT stationarity conditions as $\frac{A_{i,f}^s}{x_{i,f}^s (b_{f}^s)^2} \!\!=\!\! \vardualneqconstraintcom_{f} \!-\! \vardualeqconstraintcom_{f}^s, \forall f \!\in\! \mathcal{F}, \forall s \!\in\! \mathcal{S}$. 
\end{proof}
}
