# Supplementary material for: Joint Wireless and Edge Computing Resource Management with Dynamic Network Slice Selection
Source: arXiv:2001.07964 source file (2020-01-22)
Supplement: Supplementary file 2 [file appendix_new.tex]

\color{blue}
\begin{lemma}\label{lemm::closed_form_general}
	Let us consider the following problem 
\begin{eqnarray}
 &\min \nolimits_{\boldsymbol{b},\boldsymbol{x}} \sum \nolimits_{p \in \mathcal{S}} \sum \nolimits_{g \in \mathcal{F}} \frac{1}{b_{g}^{p}} \big(\sum \nolimits_{j \in \mathcal{O}_{g,p}}\frac{A_{j,g}^{p}}{x_{j,g}^{p}}\big)\label{eq::general_objective}\\
 \textrm{s.t.} &\sum \nolimits_{p \in \mathcal{S}}  b_{f}^{p} \leq 1, \forall f \in \mathcal{F}, \hspace{0.4cm} \label{eq::constraint_sum_of_variables_SRO}\\
 & \sum \nolimits_{j \in \mathcal{O}_{f,s}}  x_{j,f}^s \leq 1, \forall f \in \mathcal{F},\forall s \in \mathcal{S}, \hspace{0.4cm} \label{eq::constraint_sum_of_variables_slices}\\
 & b_{f}^s \geq 0, \forall f \in \mathcal{F},  \forall s \in \mathcal{S}, \label{eq::constraint_positive_variable_constraint_SRO}\\
 &x_{i,f}^s \geq 0, \forall i \in \mathcal{O}_{f,s}, \forall f \in \mathcal{F},  \forall s \in \mathcal{S}, \label{eq::constraint_positive_variable_constraint_slices}
  \end{eqnarray}
 where $A_{i,f}^s \!\in\! \mathbb{R}_{\geq 0}$ and $\mathcal{F}$, $\mathcal{S}$ and $\mathcal{O} = \cup_{g \in \mathcal{F}, p \in \mathcal{S}}\mathcal{O}_{g,p}$ are non-empty sets.
 Then, closed form solution for (\ref{eq::general_objective})-(\ref{eq::constraint_positive_variable_constraint_slices}) is given by 
 \begin{eqnarray}
     &\hat{x}_{i,f}^{s} = \frac{\sqrt{A_{i,f}^s}}{\sum \nolimits_{j \in \mathcal{O}_{f,s}}\sqrt{A_{j,f}^s}}, \forall i \in \mathcal{O}_{f,s}, \forall f \in \mathcal{F}, \forall s \in \mathcal{S}, \label{eq::optimal_coef_slices} \\
 	&\hat{b}_f^{s} = \frac{\sum \nolimits_{j \in \mathcal{O}_{f,s}}\sqrt{A_{j,f}^s}}{\sum \nolimits_{p \in \mathcal{S}}\sum \nolimits_{j \in \mathcal{O}_{f,p}}\sqrt{A_{j,f}^{p}}}, \forall f \in \mathcal{F}, \forall s \in \mathcal{S}. \label{eq::optimal_coef_SRO}
	\end{eqnarray}
 \end{lemma}
\begin{proof}
By inspecting the leading minors of the Hessian matrix of the objective function it is easy to show that the matrix is positive semidefinite on the domain defined by (\ref{eq::constraint_sum_of_variables_SRO})-(\ref{eq::constraint_positive_variable_constraint_slices}), and thus problem (\ref{eq::general_objective})-(\ref{eq::constraint_positive_variable_constraint_slices}) is convex. Therefore, the optimal solution of the problem must satisfy the Karush–Kuhn–Tucker (KKT)
conditions and thus we can formulate the corresponding Lagrangian dual problem. To do so, let us introduce non-negative Lagrange multiplier vectors $\boldsymbol{\alpha} = (\alpha_{f})_{f \in \mathcal{F}}$, $\boldsymbol{\beta} = (\beta_{f}^s)_{f \in \mathcal{F}, s \in \mathcal{S}}$, $\boldsymbol{\gamma} = (\gamma_{f}^s)_{f \in \mathcal{F}, s \in \mathcal{S}}$ and $\boldsymbol{\delta} = (\delta_{i,f}^s)_{i \in \mathcal{O}_{f,s},f \in \mathcal{F}, s \in \mathcal{S}}$  for constraints (\ref{eq::constraint_sum_of_variables_SRO})-(\ref{eq::constraint_positive_variable_constraint_slices}), respectively. Next, let us define the Lagrangian dual problem corresponding to problem (\ref{eq::general_objective})-(\ref{eq::constraint_positive_variable_constraint_slices}) as $\max \limits_{\boldsymbol{\alpha}, \boldsymbol{\beta}, \boldsymbol{\gamma},\boldsymbol{\delta}\succeq 0} \min \limits_{\boldsymbol{b},\boldsymbol{x} \succeq 0} \varlagrangian(\boldsymbol{b},\boldsymbol{x},\boldsymbol{\alpha}, \boldsymbol{\beta}, \boldsymbol{\gamma},\boldsymbol{\delta})$, where the Lagrangian is given by
\vspace{-0.3cm}
\begin{eqnarray}\label{eq::lagrangian_function_general}\nonumber
 &\varlagrangian(\boldsymbol{b},\boldsymbol{x},\boldsymbol{\alpha}, \boldsymbol{\beta}, \boldsymbol{\gamma},\boldsymbol{\delta})= \sum \limits_{p \in \mathcal{S}} \sum \limits_{g \in \mathcal{F}} \frac{1}{b_{g}^p} \big(\sum \limits_{j \in \mathcal{O}_{g,p}}\frac{A_{j,g}^p}{x_{j,g}^p}\big)+\\\nonumber
  &\hspace{-0.2cm}\sum_{g \in \mathcal{F}} \alpha_g (\sum_{p \in \mathcal{S}}  b_{g}^{p} - 1) + \sum \limits_{g \in \mathcal{F}} \sum \limits_{p \in \mathcal{S}}\! \beta_{g}^p \big(\sum \limits_{j \in \mathcal{O}_{g,p}}\!\!x_{j,g}^p - 1) \big)  -\\\nonumber
  &\sum_{g \in \mathcal{F}} \sum_{p \in \mathcal{S}} \gamma_g^{p}b_{g}^{p}- \sum \limits_{g \in \mathcal{F}} \sum \limits_{p \in \mathcal{S}} \sum \limits_{j \in \mathcal{O}_{g,p}} \delta_{j,g}^p x_{j,g}^p.\nonumber
 \end{eqnarray}
 Now, we can express the KKT conditions as follows
 \begin{eqnarray}
  \textrm{\scriptsize \textbf{stationarity:}} & \hspace{-0.4cm}\sum \limits_{j \in \mathcal{O}_{f,s}}\!\!\!\!\!\frac{A_{j,f}^{s}}{x_{j,f}^{s}}\frac{1}{(b_{f}^s)^2} \!\!=\!\! \alpha_{f} \!-\! \gamma_{f}^s, \forall f \!\in\! \mathcal{F}, \! s \!\in\! \mathcal{S},  \label{KKT::stationarity_SRO}\\
  &\hspace{-0.35cm}\frac{A_{i,f}^s}{b_{f}^s(x_{i,f}^s)^2}\!\!=\!\! \beta_{f}^s \!-\! \delta_{i,f}^s, 
 \!\forall \!f \!\!\in\!\! \mathcal{F}, \!s \!\!\in\! \mathcal{S}, \!i \!\in\!\! \mathcal{O}_{f,s}, \label{KKT::stationarity_slices}\\
   \textrm{\scriptsize \textbf{prim. feasibility:}} &\hspace{-4.1cm} (\ref{eq::constraint_sum_of_variables_slices})-(\ref{eq::constraint_positive_variable_constraint_SRO}), \label{KKT::primal_feasibility}\\
  \textrm{\scriptsize \textbf{dual feasibility:}} &\hspace{-3.7cm}\boldsymbol{\alpha}, \boldsymbol{\beta}, \boldsymbol{\gamma},\boldsymbol{\delta} \succeq 0, \label{KKT::dual_feasibility}\\
  \textrm{\scriptsize \textbf{comp. slackness:}} &\hspace{-2.4cm}\alpha_{f}(\sum \limits_{p \in \mathcal{S}}  b_{f}^{p} - 1),\! \forall f \!\in\! \mathcal{F},  \label{KKT::complementary_slackness_1}\\
  \textrm{\scriptsize \textbf{\color{white}slackness:\color{black}}} &\hspace{-0.6cm}\beta_{f}^s(\sum \limits_{j \in \mathcal{O}_{f,s}}\!\!\!\!x_{j,f}^s - 1) = 0,\! \forall f \!\in\! \mathcal{F},\! s \in \mathcal{S}, \label{KKT::complementary_slackness_2}\\
  \textrm{\scriptsize \textbf{\color{white} complementary \color{black}}} &\hspace{-3.2cm}-\gamma_f^{s}b_{f}^{s} = 0,\! \forall f \!\in\! \mathcal{F},  \label{KKT::complementary_slackness_3}\\
  \textrm{\scriptsize \textbf{\color{white} slackness: \color{black}}} &\hspace{-0.9cm}-\delta_{i,f}^s x_{i,f}^s = 0,\!\forall \!f \!\in\! \mathcal{F}, \!s \!\in\! \mathcal{S}, \!i\in\! \mathcal{O}_{f,s}. \label{KKT::complementary_slackness_4}
  \end{eqnarray}
  We proceed with finding $\hat{x}_{i,f}^{s}$. First, from the KKT dual feasibility condition $\boldsymbol{\delta} \!\succeq\! 0$ and complementary slackness condition (\ref{KKT::complementary_slackness_4}) we obtain that $\delta_{i,f}^s \!=\! 0$ must hold for every $f \!\in\! \mathcal{F}$, $s \!\in\! \mathcal{S}$ and $i \!\in\! \mathcal{K}_{f,s}$ as otherwise $x_{i,f}^s \!=\! 0$ would lead to infinite value of the objective function. Then, from the KKT stationarity condition (\ref{KKT::stationarity_slices}) and complementary slackness condition (\ref{KKT::complementary_slackness_2}) we obtain the expression~(\ref{eq::optimal_coef_slices}) for coefficients $\hat{x}_{i,f}^s$. Finally, by substituting expression~(\ref{eq::optimal_coef_slices}) into the KKT stationarity condition (\ref{KKT::stationarity_SRO}) and by following the same approach as for expressing $x_{i,f}^*$ we obtain the expression~(\ref{eq::optimal_coef_SRO}) for coefficients $\hat{b}_{f}$, which proves the result.
\end{proof}
\begin{lemma}\label{lemm::closed_form_slices}
	Let us consider the following problem 
\begin{eqnarray}
 &\min \nolimits_{\boldsymbol{x}} \sum \nolimits_{p \in \mathcal{S}} \sum \nolimits_{g \in \mathcal{F}} \frac{1}{b_{g}^{p}} \big(\sum \nolimits_{j \in \mathcal{O}_{g,p}}\frac{A_{j,g}^{p}}{x_{j,g}^{p}}\big)\label{eq::objective_slices}\\
 \textrm{s.t.} & (\ref{eq::constraint_sum_of_variables_slices}) \text{ and } (\ref{eq::constraint_positive_variable_constraint_slices}), \label{eq::slices_both_constraint}
  \end{eqnarray}
 where $b_{g}^p \!\in\! \mathbb{R}_{> 0}$ are positive constants for every $g \in \mathcal{F}$ and $p \in \mathcal{S}$.
 Then, closed form solution for (\ref{eq::objective_slices})-(\ref{eq::slices_both_constraint}) is given by~(\ref{eq::optimal_coef_slices}).
\end{lemma}
\begin{proof}
	The result can be proved by following the same approach presented in the proof of Lemma~\ref{lemm::closed_form_general}.
\end{proof}
\begin{lemma}\label{lemm::closed_form_SRO}
	Let us consider the following problem 
\begin{eqnarray}
&\min \nolimits_{\boldsymbol{b}} \sum \nolimits_{p \in \mathcal{S}} \sum \nolimits_{g \in \mathcal{F}} \frac{1}{b_{g}^p} \big(\sum \nolimits_{i \in \mathcal{O}_{g,p}}\sqrt{A_{i,g}^p}\big)^2\label{eq::SRO_objective}\\
\textrm{s.t.} & (\ref{eq::constraint_sum_of_variables_SRO}) \text{ and } (\ref{eq::constraint_positive_variable_constraint_SRO}), \label{eq::SRO_both_constraint}
\end{eqnarray}
	obtained by substituting (\ref{eq::optimal_coef_slices}) into (\ref{eq::general_objective}).
	Then, closed form solution for (\ref{eq::SRO_objective})-(\ref{eq::SRO_both_constraint}) is given by~(\ref{eq::optimal_coef_SRO}).
\end{lemma}
\begin{proof}
	The result can be proved by following the same approach presented in the proof of Lemma~\ref{lemm::closed_form_general}.
\end{proof}
\color{black}
